# Supplementary material for: In-Context Learning User Simulators for Task-Oriented Dialog Systems
Source: arXiv:2306.00774 source file (2023-06-01)
Supplement: Supplementary file 1 [file full_results_appendix.tex]

\begin{table*}[ht]
\centering\small
% \begin{tabular}{llllllllllll}
\begin{tabular}{p{1.2in}p{0.3in}p{0.3in}p{0.25in}p{0.25in}p{0.3in}p{0.3in}p{0.3in}p{0.3in}p{0.3in}p{0.3in}p{0.3in}}
fuuuuul results & Success & Fulfill & Uni-grams & Bi-grams & Tri-grams & Avg utt length & Entropy tokens & Cond entropy & MSTTR & HDD & MTLD \\
  \hline
% references: have to adjust them manually after running
% python scripts/calculate_diversity.py --dataset_path data/multiwoz/train.json --data-key usr --sample 200
% python tutorials/user_simulator_script_ours.py --user-simulator rulebased --total-dialog 200
ref: sampled train & 1,345 & 16,959 & 919 & 4,505 & 7,678 & 12.6 & 7.3 & 3.0 & 0.76 & 0.78 & 61.0 \\
ref: rule based &  1,191 & 20,671 & 527 & 2,140 & 3,867 & 17.4 & 6.9 & 2.5 & 0.72 & 0.75 & 46.9 \\
  \hline
% copy paste experimental results here:
google\_flan-t5-xl\_rss &  937 & 11,986 & 760 & 3,122 & 4,993 & 12.8 & 7.1 & 2.6 & 0.68 & 0.75 & 43.0 \\
azure\_openai\_gpt-35-turbo\_rss & 1,457 & 23,580 & \textbf{981} & \textbf{4,350} & \textbf{7,661} & 16.2 & \textbf{7.4} & \textbf{2.9} & \textbf{0.73} & \textbf{0.79} & \textbf{53.6} \\

% copy paste end
\end{tabular}
\caption{Placeholder for full results: goal fulfillment, diversity, all experimental conditions. Each model generated the same 200 conversations. }
\label{tab:full_results}
\end{table*}
